# Supplementary material for: Performance Evaluation of Dynamic Metasurface Antennas: Impact of Insertion Losses and Coupling
Source: arXiv:2206.13245 source file (2022-06-27)
Supplement: Supplementary file 1 [file appendix.tex]

The gradient of $f(\mat{Y}_\text{s}^\text{im})$ in \eqref{eq:P2} is calculated using complex matrix differentials theory \cite{Hjrungnes2011}. For the sake of clarity in the notation, throughout this appendix the subindex $(\cdot)_\text{dma}$ in $\mat{H}^\dagger_\text{dma}$ is omitted. Hence, applying the chain rule for differentials \cite[Eq. (3.35)]{Hjrungnes2011} in \eqref{eq:P2}, we obtain that
\begin{align}
    \dif\,f(\mat{Y}_\text{s}^\text{im}) =& \text{Tr}\left\{\Re{\dif\,\mat{Y}_\text{q}}\mat{H}^\dagger(\mat{H}^\dagger)^H \right\} \notag \\
    &+ \text{Tr}\left\{\Re{\mat{Y}_\text{q}}\dif\,(\mat{H}^\dagger(\mat{H}^\dagger)^H) \right\}. \label{eq:dif_f}
\end{align}

Applying again basic operations for differentials, $\dif\,\mat{Y}_\text{q}$ is calculated as
\begin{align}
    \dif\,\mat{Y}_\text{q} = \dif\,\p{(\mat{I}_N-\bm{\Gamma}^H\bm{\Gamma})^{-1}}\mat{Y}_\text{p} + \mat{D}\dif\,\mat{Y}_\text{p}, \label{eq:dif_Yq}
\end{align}
where $\mat{D}$ defined as in \eqref{eq:D} and
\begin{equation}
    \dif\,\mat{Y}_\text{p} = \left(j\mat{Y}_\text{st}^T\mat{A}^{-1}\dif\,\mat{Y}^\text{im}_\text{s}\mat{A}^{-1}\mat{Y}_\text{st}\right).
\end{equation}
On the other hand, we have
\begin{align}
    \dif\,(\mat{I}_N-\bm{\Gamma}^H\bm{\Gamma})^{-1} =& \mat{D} \left(\left[(\mat{I}_N-\bm{\Gamma})(\dif\,\mat{Y}_\text{p}\circ\mat{I})\mat{C}\right]^H\bm{\Gamma}\bm{\Gamma}^H\right. \notag \\
    &\times\left.\left[(\mat{I}_N-\bm{\Gamma})(\dif\,\mat{Y}_\text{p}\circ\mat{I})\mat{C}\right]\right)\mat{D},
\end{align}
where $\mat{C}$ is defined in \eqref{eq:C}. Note that, according to the simplifying assumption in Section \ref{subsec:DMA_system_model}, we enforce $\mat{Y}_\text{p}$ to be a diagonal matrix for the calculation of $\mat{\Gamma}$.

Regarding the term $\mat{H}^\dagger(\mat{H}^\dagger)^H$, using again the chain rule yields
\begin{equation}
    \dif\,\mat{H}^\dagger(\mat{H}^\dagger)^H = (\dif\,\mat{H}^\dagger)(\mat{H}^\dagger)^H + \mat{H}^\dagger(\dif\,\mat{H}^\dagger)^H,
\end{equation}
where the differential of the pseudo-inverse is readily obtained from \cite[Eq. (3.64)]{Hjrungnes2011} as (note that we have relabeled $\mat{H}_\text{eq}^\text{dma}$ as simply $\mat{H}$)
\begin{align}
    \dif\,\mat{H}^\dagger = (\mat{I}_N-\mat{H}^\dagger\mat{H})(\dif\,\mat{H})^H(\mat{H}^\dagger)^H\mat{H}^\dagger-\mat{H}^\dagger (\dif\,\mat{H})\mat{H}^\dagger 
\end{align}
since, in our case, $\mat{H}\mat{H}^\dagger= \mat{I}_M$ as long as $M\leq N$. The differential of $\mat{H}$ is computed in the same way as that of $\mat{Y}_\text{p}$, and hence after some algebraic manipulations we obtain
\begin{align}
    \dif\,&\mat{H}^\dagger = -j\mat{H}^\dagger\widetilde{\mat{Y}}_\text{rs}\mat{A}^{-1}(\dif\,\mat{Y}_\text{s}^\text{im})\mat{A}^{-1}\mat{Y}_\text{st} \mat{H}^\dagger \notag \\
    &+ (\mat{I}-\mat{H}^\dagger\mat{H})(\widetilde{\mat{Y}}_\text{rs}\mat{A}^{-1}(\dif\,\mat{Y}_\text{s}^\text{im})\mat{A}^{-1}\mat{Y}_\text{st})^H(\mat{H}^\dagger)^H\mat{H}^\dagger,
\end{align}
with $\mat{A}^{-1}$ as in \eqref{eq:A}. From \eqref{eq:dif_f} and the expressions for the respective differentials, the derivative of $f(\mat{Y}_\text{s}^\text{im})$ w.r.t. $\mat{Y}_\text{s}^\text{im}$ is obtained applying \cite[Eqs. (4.39)-(4.44)]{Hjrungnes2011}, yielding the following relation
\begin{equation}
    \dif f(\mat{Y}_\text{s}^\text{im}) = \text{Tr}\left\{\mat{X}\dif\,\mat{Y}_\text{s}^\text{im}\right\} \Rightarrow \der{f(\mat{Y}_\text{s}^\text{im})}{\mat{Y}_\text{s}^\text{im}} = \mat{X}^T. \label{eq:dif_der_relation}
\end{equation}

Then, introducing the differentials in \eqref{eq:dif_f}, applying the rotational property of the trace and $\text{Tr}\left\{\mat{X}(\mat{Y}\circ\mat{Z})\right\} = \text{Tr}\left\{(\mat{X}\circ\mat{Y}^T)\mat{Z}\right\}$ (given the proper matrix dimensions), we can rewrite \eqref{eq:dif_f} in the same form as  \eqref{eq:dif_der_relation}, yielding \eqref{eq:Gradient}.
